# Supplementary material for: Mitigating Spurious Correlations in Weakly Supervised Semantic Segmentation via Cross-architecture Consistency Regularization
Source: arXiv:2507.21959 source file (2025-07-29)
Supplement: Supplementary file 1 [file appendix-a.tex]

\chapter{First appendix}
\label{First appendix}
\phantomsection

\begin{figure}[H]
    \centering
    \includegraphics[width=0.95\linewidth]{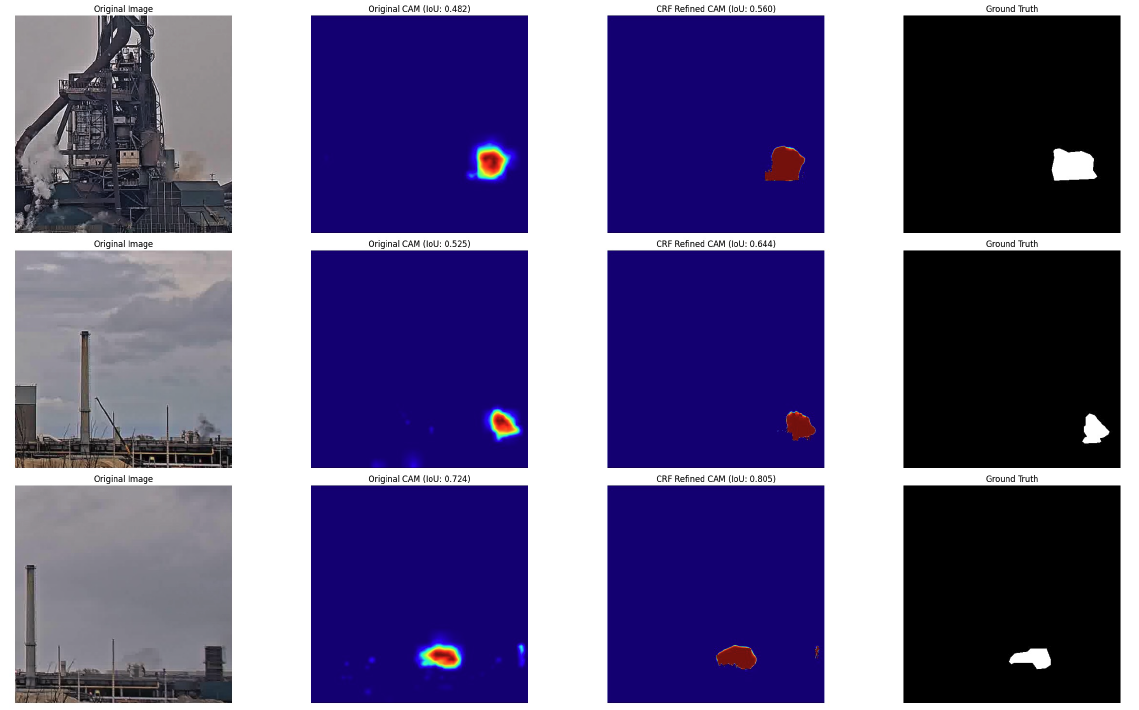}
    \caption{CRF Refinement}
    \label{fig:CRF}
\end{figure}

\textbf{Cross-view Consistency:}~From Table~\ref{tab:consistency table}
We can see both improvement and drop of mIOU occurs when  consistency loss is applied,~indicating inconsistent guidance.
Visual inspection of CAMs between original and augmented views reveals minimal activation shifts,~we argue that the discrepancy is relatively low,~suggests that current consistency losses fail to enforce meaningful spatial constraints when feature variations are subtle.

\begin{table}[ht]
\centering
\caption{Logits-level consistency of augmented view.{-} means no consistency loss applied.}
\label{tab:consistency table}
\vspace{-0.5em}
\begin{tabular}{lccc}
\toprule
\textbf{View} & \textbf{Backbone} & \textbf{Level} &\textbf{mIOU}\\
\midrule
Vanilla & ResNet101& {-}&21.29\\
Augmented& ResNet101&Logit &29.73\\
Vanilla & ResNet50& {-}&25.49\\
Augmented& ResNet50&Logit &24.61\\
\midrule 
\end{tabular}
\end{table}

\begin{table}[htbp]
\centering
\caption{Impact of hyper-parameters(co-training+cosine+channel+without feature projection).Gray rows indicate default settings.}
\label{tab:hyperparam_impact}
\begin{subtable}[t]{0.32\textwidth}
\centering
\begin{tabular}{lcc}
\hline
\textbf{Points} & \textbf{Seed} & \textbf{SAM}  \\ 
\hline
32 & 38.49  &  43.13 \\
\rowcolor{gray!20}
48& 38.49  & 43.20  \\
64& 38.49  &   43.12 \\

\hline
\end{tabular}
\caption{Points per side}
\label{subtab:block}
\end{subtable}
\hfill
\begin{subtable}[t]{0.32\textwidth}
\centering
\begin{tabular}{lcc}
\hline
\textbf{Layer} & \textbf{Seed} & \textbf{mIOU} \\
\hline
\rowcolor{gray!20}
-5,-4,-2 & 38.49 & 46.91 \\
-4,-2 & 38.49 &  45.99\\
-4,-2,-1& 38.49 &  45.11\\
-4,-1 & 38.49&  46.90\\
\hline
\end{tabular}
\caption{Layer chosen for fusion}
\label{subtab:size}
\end{subtable}
\hfill
\begin{subtable}[t]{0.32\textwidth}
\centering
\begin{tabular}{lcc}
\hline
\textbf{Scaling factor} & \textbf{Seed} & \textbf{dCRF} \\
\hline

8   &  38.49& 34.38 \\
16  & 38.49 &  41.32\\
\rowcolor{gray!20}
32  & 38.49 &44.20\\
36  & 38.49 &44.13\\
48 & 38.49 &43.27\\

\hline
\end{tabular}
\caption{Experiments with CRF parameter}
\label{subtab:momentum}
\end{subtable}

\vspace{0.2cm}
\footnotesize
\end{table}

\begin{figure}[htbp]
\centering
\setlength{\tabcolsep}{2pt} % Adjust space between columns
 % Adjust space between rows
\begin{tabular}{c c c c}
\textbf{scale:0.5} & \textbf{scale:1.0} & \textbf{scale:1.5} & \textbf{Fusion} \\

\includegraphics[width=0.22\textwidth]{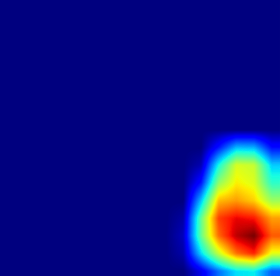} & 
\includegraphics[width=0.22\textwidth]{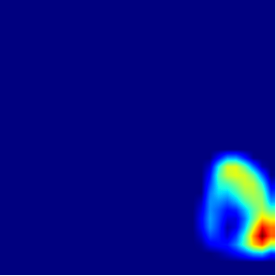} &
\includegraphics[width=0.22\textwidth]{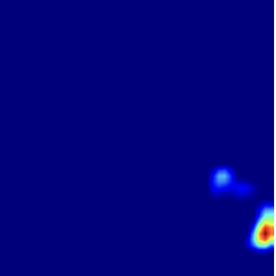} &
\includegraphics[width=0.22\textwidth]{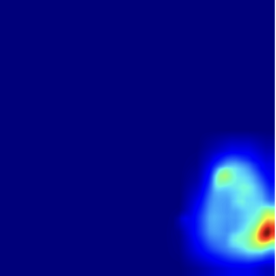} \\
\end{tabular}

\caption{Multi scale(Resnet101)}
\label{fig:method_comparison}
\end{figure}

% \subsubsection{Multi-stage learning strategy   }
% \textbf{Dynamically adjust loss weight}:
% \subsubsection{}
% Vision Transformers benefit from:smooth LR decay and Warmup phases (start slow, then increase LR).
% For scheduler,StepLR is not ideal as it suddenly drops which is unstable.

% Different learning rates leading to different attention paths.
% Whether it converges at all.  
% We run learning rate range test.By experiment,when the learning rate is above 1e-3,the model collapses into random guessing.
% That’s why Grad-CAM or attention visualization looks good in one run , but not another,despite same architecture and data.
% From figure\ref{fig:lr},we can see that the loss starts dropping quickly around 1e-5,and reaches its steepest descent between 1e-4 and 3e-4.
\begin{figure}
    \centering
    \includegraphics[width=0.5\linewidth]{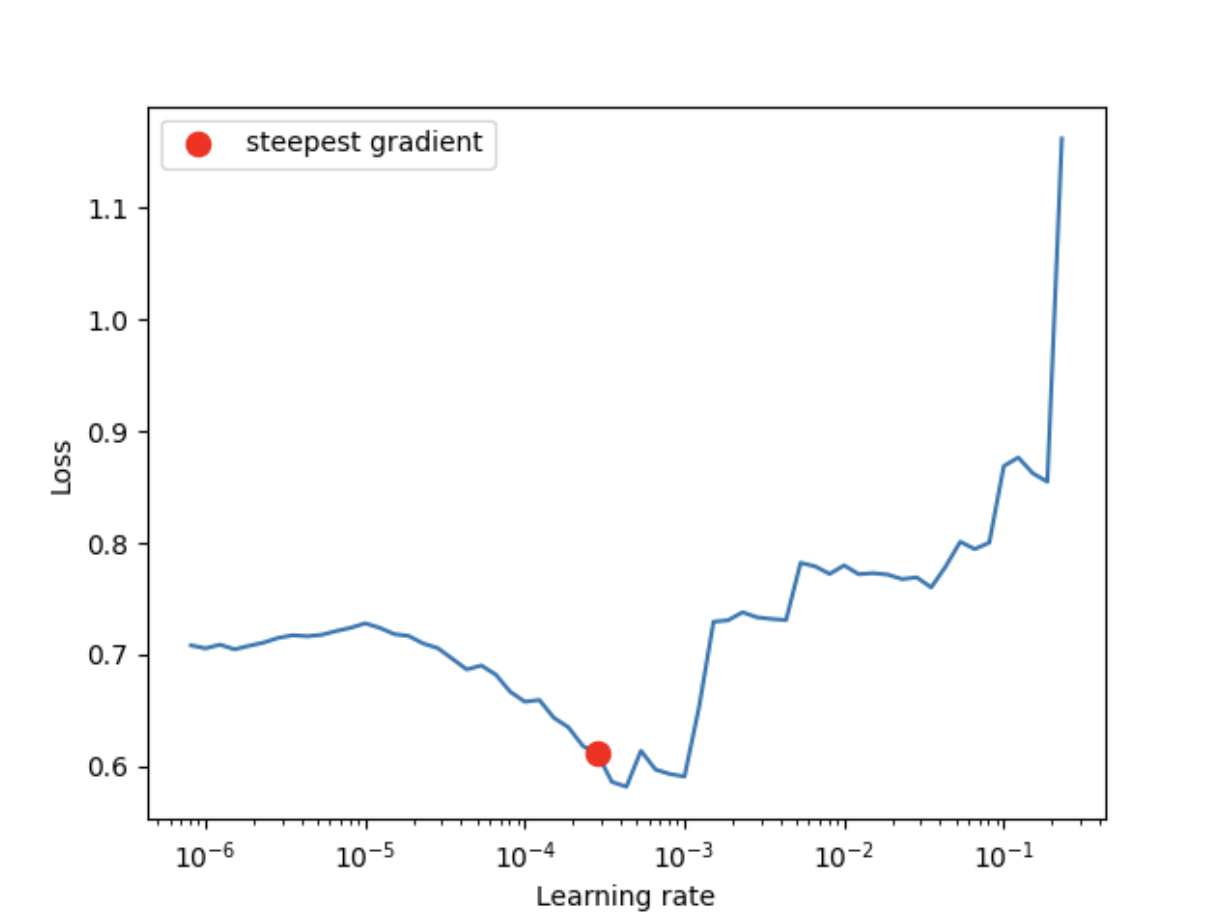}
    \caption{Learning rate range test(ViT)}
    \label{fig:lr}
\end{figure}

\begin{figure}
    \centering
    \includegraphics[width=0.5\linewidth]{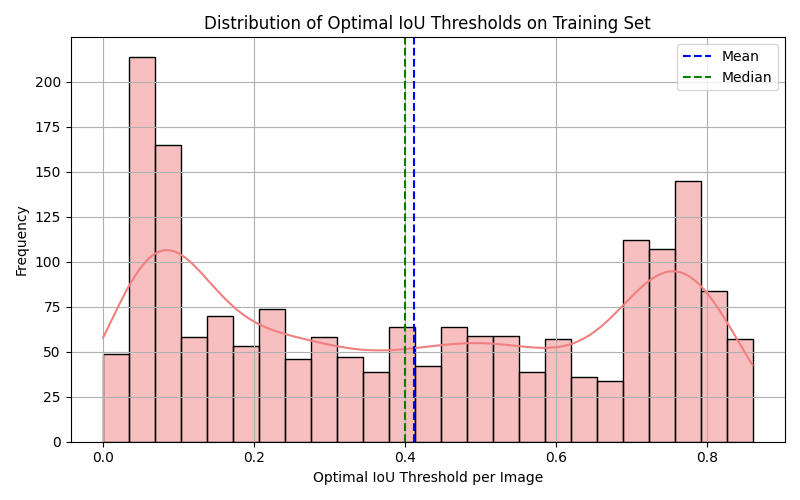}
    \caption{Optimal threshold for ResNet.}
    \label{fig:}
\end{figure}
\begin{figure}
    \centering
    \includegraphics[width=0.5\linewidth]{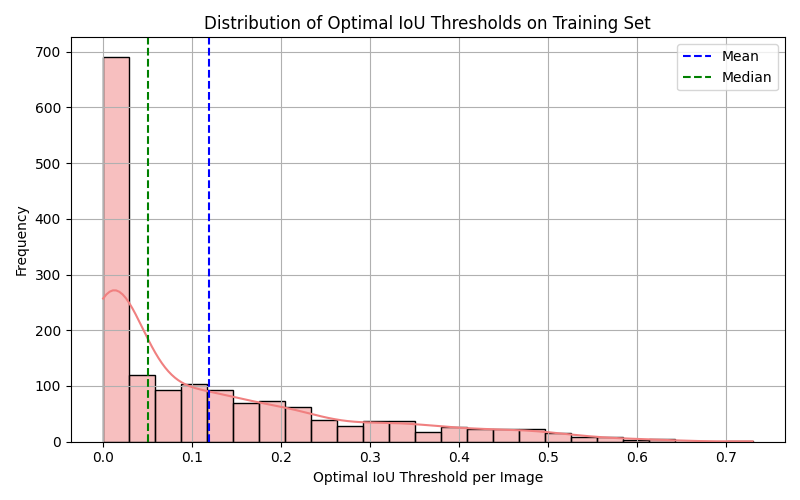}
    \caption{Optimal threshold for ViT.}
    \label{fig:}
\end{figure}

% The class tokens are visualized using t-SNE in \ref{fig:t-sne}.

% The similarity between original and augmented cls embedding is 0.911 before introduce contrastive loss.
% add 97.95%
%
\begin{figure}
    \centering
    \includegraphics[width=0.85\linewidth]{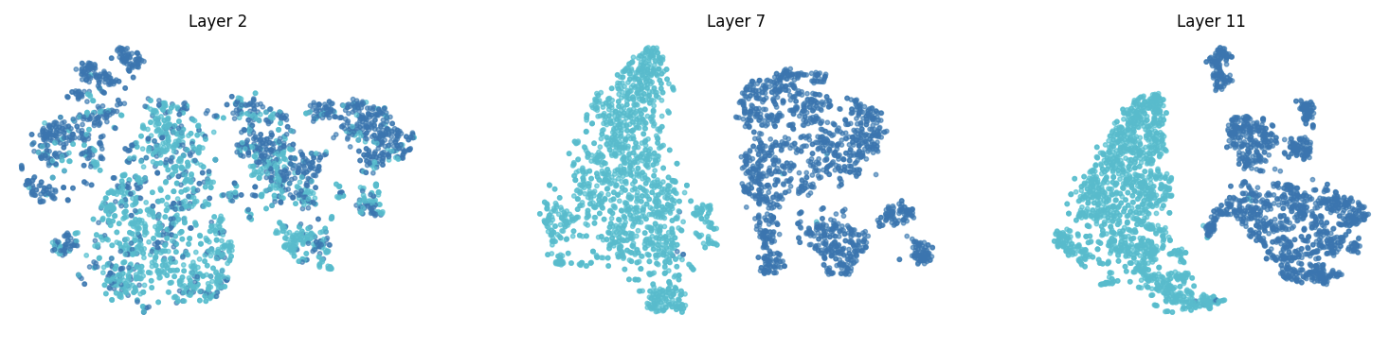}
    \caption{t-SNE of cls token for differnet layer}
    \label{fig:enter-label}
\end{figure}

\begin{figure}
    \centering
    \includegraphics[width=0.85\linewidth]{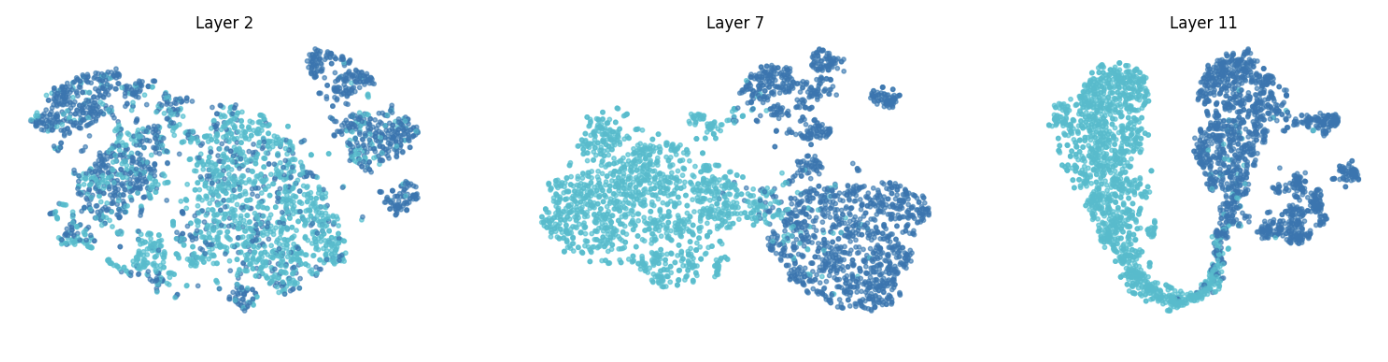}
    \caption{t-SNE of cls token for aug}
    \label{fig:tsne_aug}
\end{figure}

\begin{figure}
    \centering
    \includegraphics[width=0.3\linewidth]{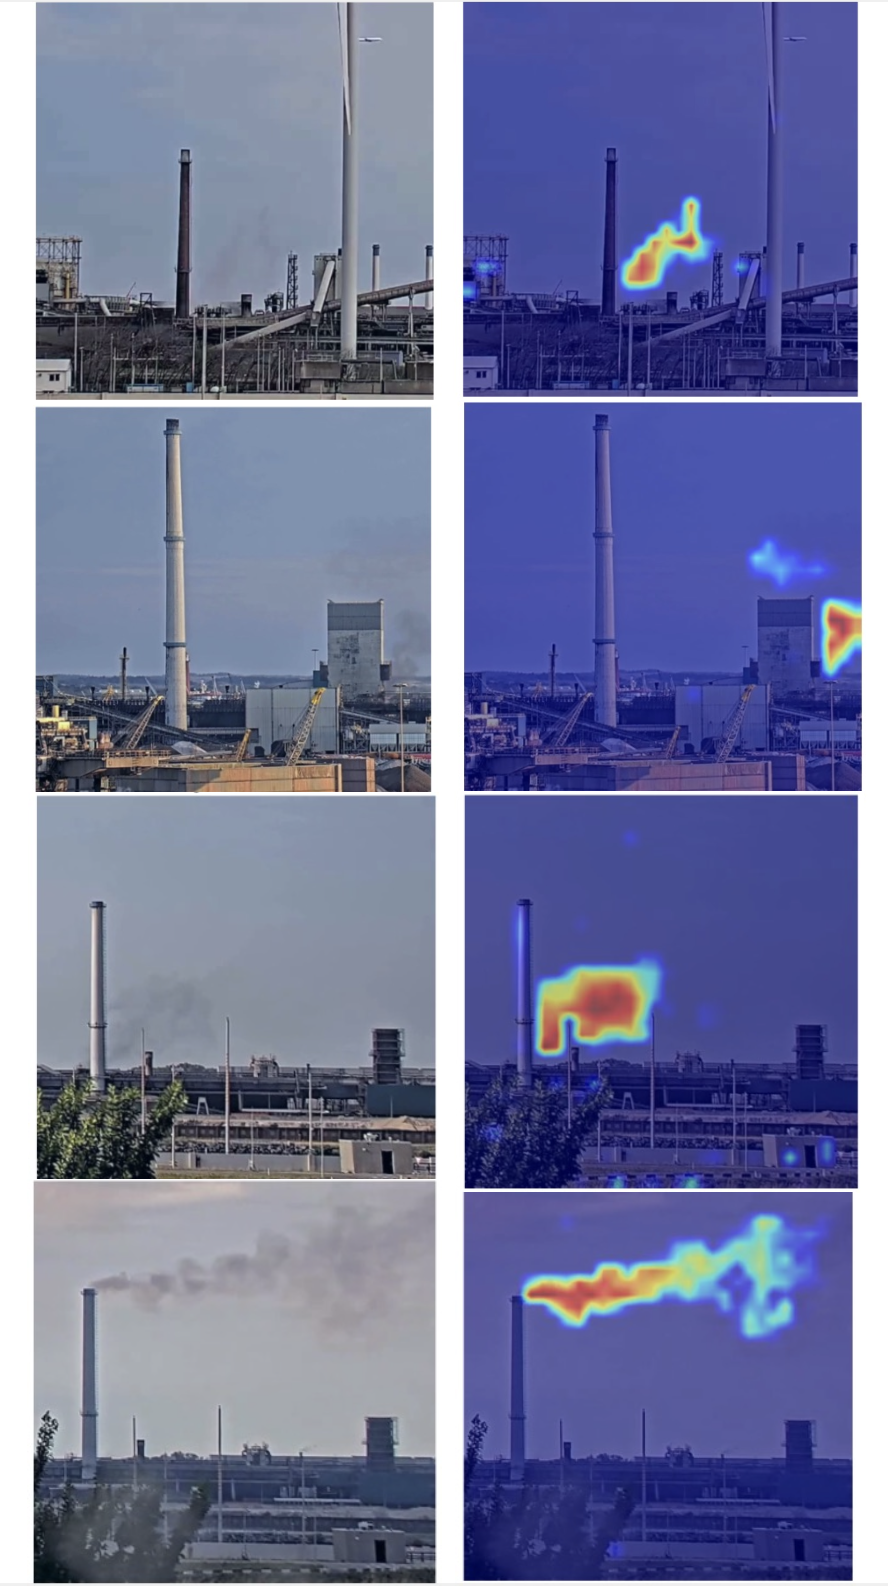}
    \caption{Sample results of visualization of localization maps on our train set.}
    \label{fig:enter-label}
\end{figure}

% \begin{figure}[htbp]
%     \centering
    
%     % 第一幅图
%     \begin{subfigure}[b]{0.75\textwidth}
%         \includegraphics[width=\textwidth]{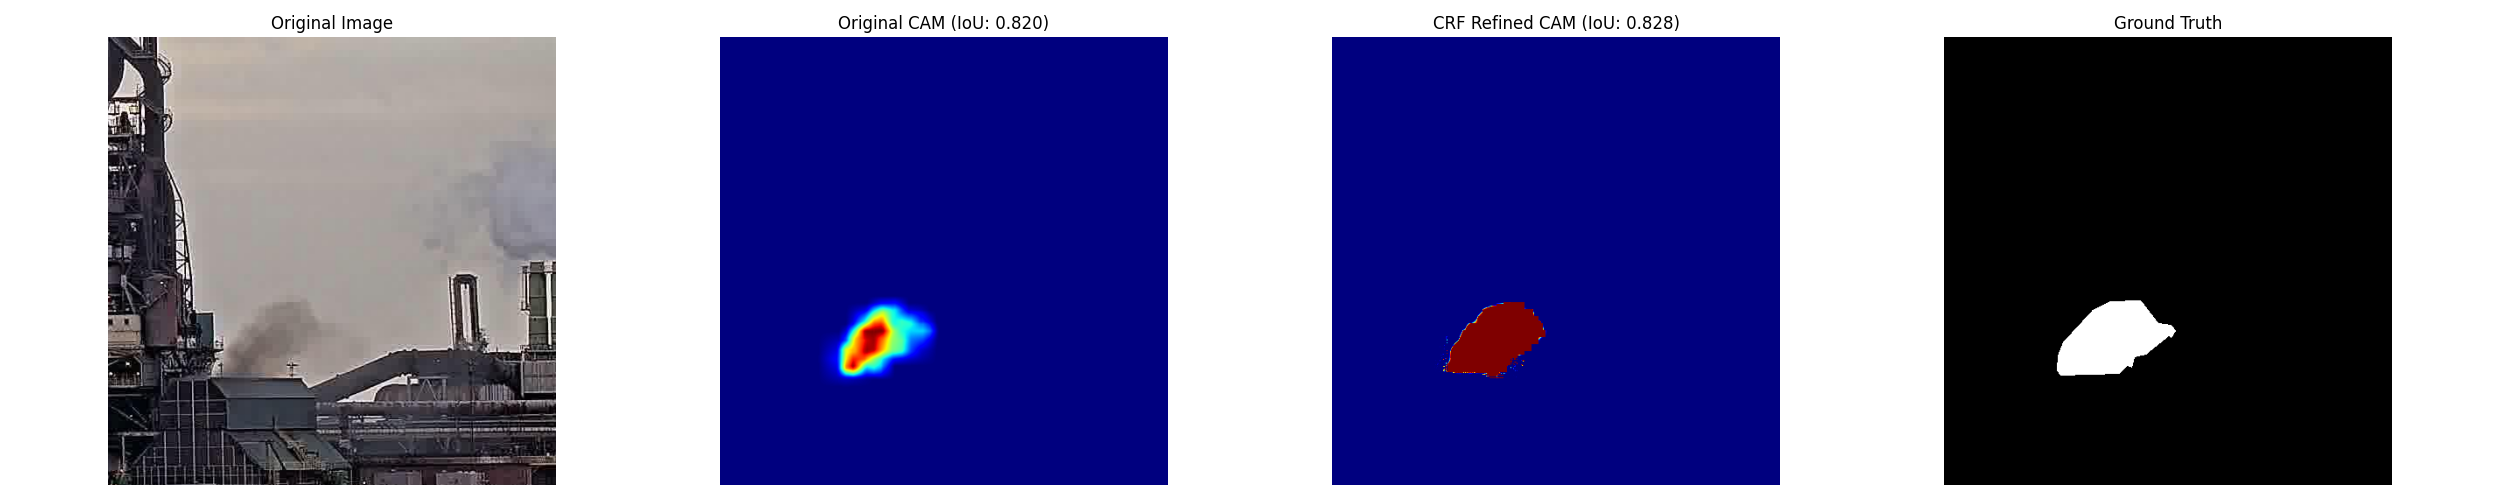}
%         \caption{CRF post process}
%         \label{fig:crf}
%     \end{subfigure}
%     \hfill  % 分隔符，自动调整间距
    
%     % 第二幅图
%     \begin{subfigure}[b]{0.75\textwidth}
%         \includegraphics[width=\textwidth]{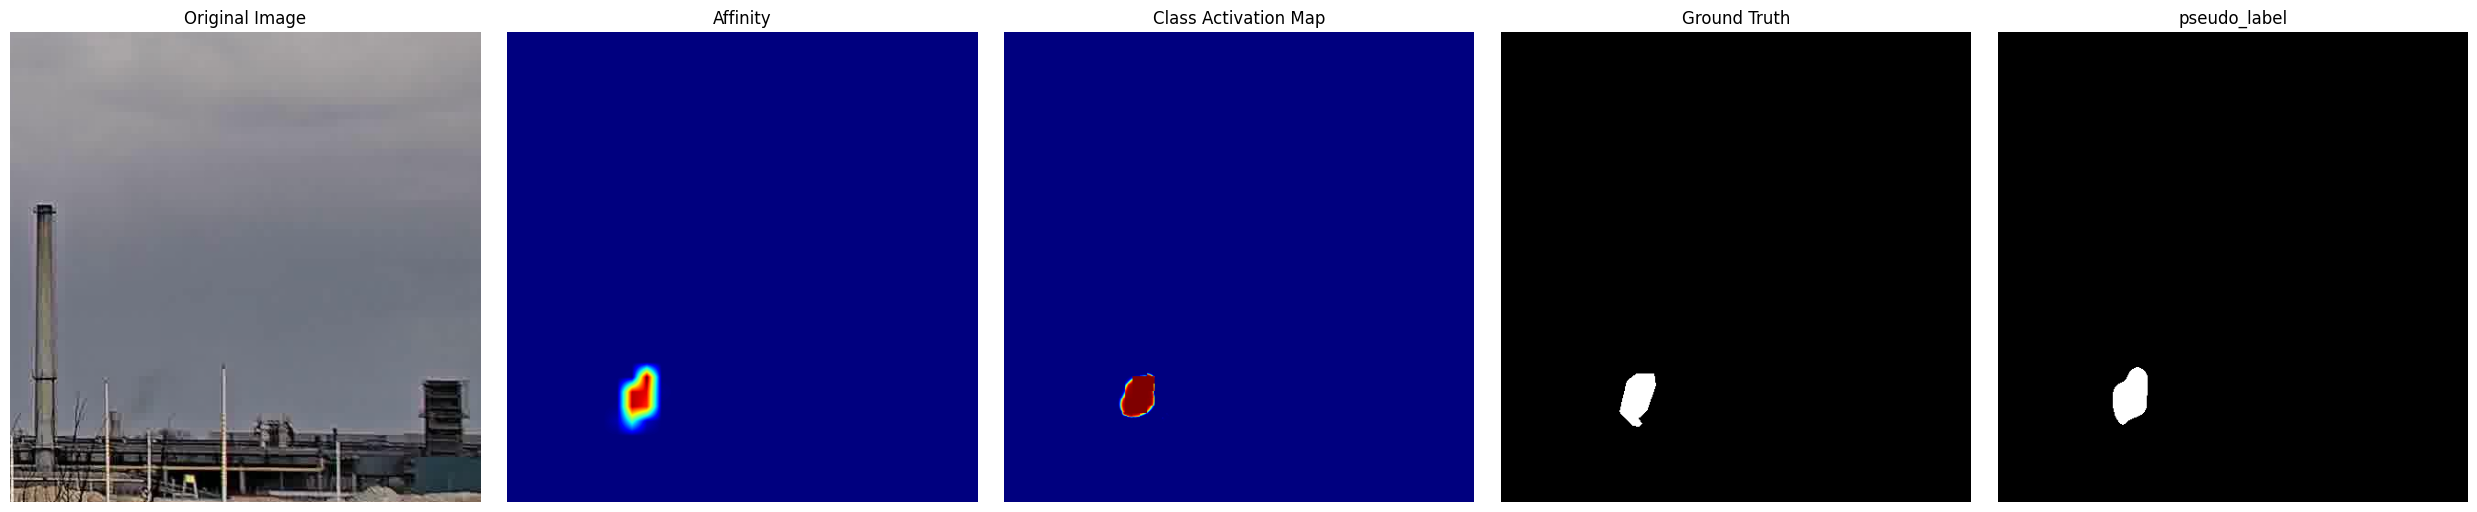}
%         \caption{Affinity Random Walk}
%         \label{fig:affinity}
%     \end{subfigure}
%     \hfill
    
%     % 第三幅图
%     \begin{subfigure}[b]{0.75\textwidth}
%         \includegraphics[width=\textwidth]{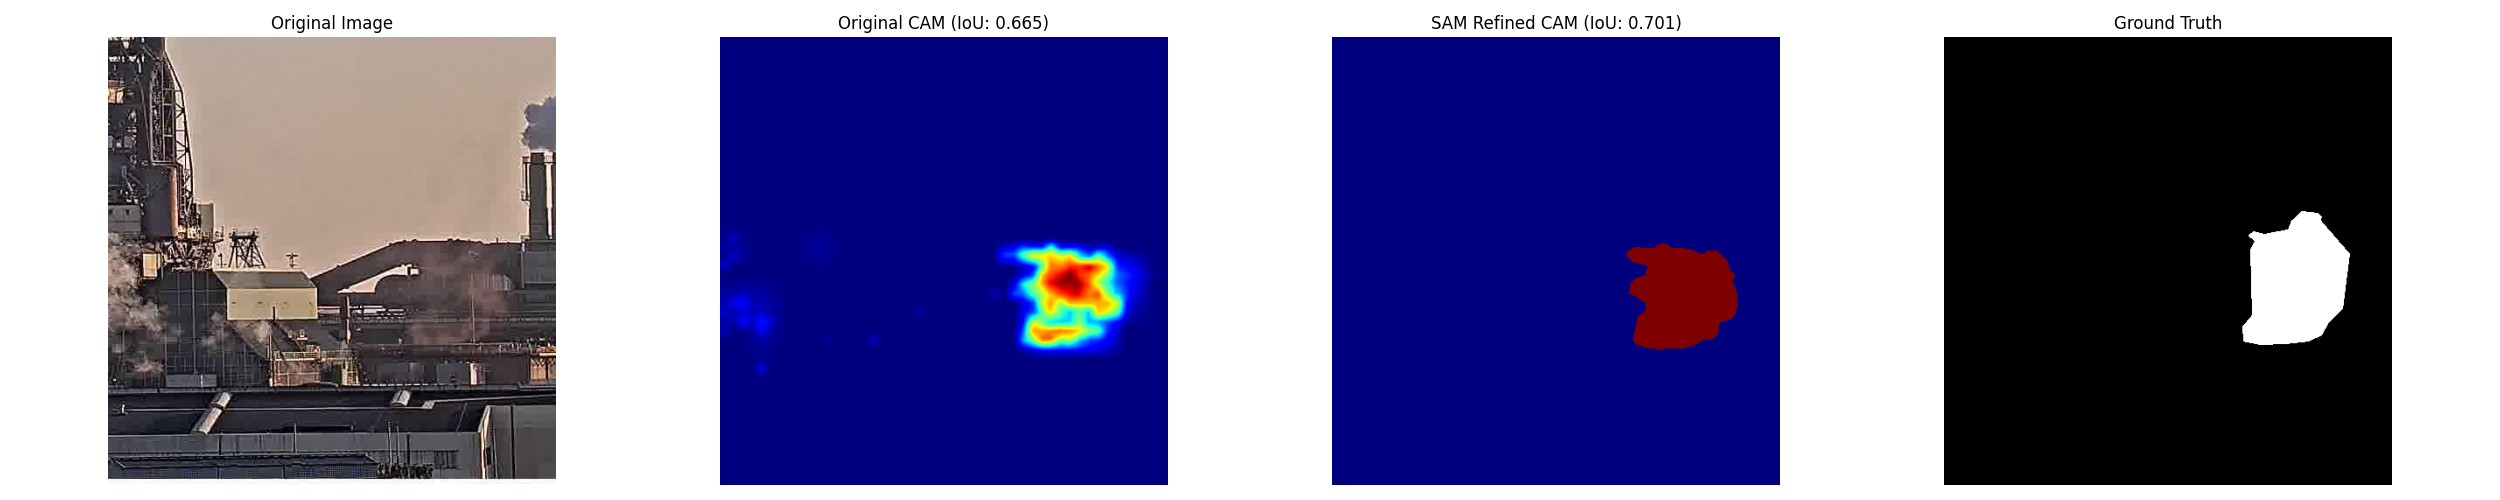}
%         \caption{SAM-enhanced}
%         \label{fig:sam}
%     \end{subfigure}
    
%     \caption{Comparison of Post-processing Methods}
%     \label{fig:methods_comparison}
% \end{figure}
