# Supplementary material for: Mitigating Spurious Correlations in Weakly Supervised Semantic Segmentation via Cross-architecture Consistency Regularization
Source: arXiv:2507.21959 source file (2025-07-29)
Supplement: Supplementary file 2 [file versicherung.tex]

\chapter*{Eidesstattliche Versicherung}

Hiermit versichere ich an Eides statt, dass ich die vorliegende Arbeit im Studiengang ......... selbstständig verfasst und keine anderen als die angegebenen Hilfsmittel – insbesondere keine im Quellenverzeichnis nicht benannten Internet-Quellen – benutzt habe. Alle Stellen, die wörtlich oder sinngemäß aus Veröffentlichungen entnommen wurden, sind als solche kenntlich gemacht. Ich versichere weiterhin, dass ich die Arbeit vorher nicht in einem anderen Prüfungsverfahren eingereicht habe und die eingereichte schriftliche Fassung der auf dem elektronischen Speichermedium entspricht.\newline

\noindent
Einer Veröffentlichung der vorliegenden Arbeit in der zuständigen Fachbibliothek des Fachbereichs stimme ich zu.\newline

\vspace{25mm}

%  The aligning options are m for middle, p for top and b for bottom. 
\noindent
\begin{tabular}{@{}p{2.5cm}p{3cm}p{2cm}p{7cm}}
Hamburg, den  & \hrulefill & Unterschrift: & \hrulefill \\
\end{tabular}

\begin{comment}
    Bei der Abgabe der Abschlussarbeit ist eine Versicherung an Eides statt (lt. § 59 Abs. 3 HmbHG) abzugeben:

„Hiermit versichere ich an Eides statt, dass ich die vorliegende Arbeit im Studiengang ...*) selbstständig verfasst und keine anderen als die angegebenen Hilfsmittel – insbesondere keine im Quellenverzeichnis nicht benannten Internet-Quellen – benutzt habe. Alle Stellen, die wörtlich oder sinngemäß aus Veröffentlichungen entnommen wurden, sind als solche kenntlich gemacht. Ich versichere weiterhin, dass ich die Arbeit vorher nicht in einem anderen Prüfungsverfahren eingereicht habe und die eingereichte schriftliche Fassung der auf dem elektronischen Speichermedium entspricht.“             *) bitte Ihren Studiengang und Abschluss eintragen

Die Angabe zur Veröffentlichung in der Fachbibliothek können Sie direkt in die Versicherung mit einbeziehen:

"Einer Veröffentlichung der vorliegenden Arbeit in der zuständigen Fachbibliothek des Fachbereichs stimme ich zu/stimme ich nicht zu."

Bitte drucken Sie diese Versicherung in jedem Exemplar am Ende ab und unterschreiben Sie diese mit der Angabe von Ort und Datum.
\end{comment}
